# Supplementary material for: Laterally Extended States of Interlayer Excitons in Reconstructed MoSe$_2$/WSe$_2$ Heterostructures
Source: arXiv:2411.19616 source file (2024-11-29)
Supplement: Supplementary file 1 [file SI.pdf]

# Supplementary Info
# Laterally Extended States of Interlayer Excitons in Reconstructed $MoSe_2/WSe_2$ Heterostructures

Johannes Figueiredo,[1,2] Marten Richter,[3,*] Mirco Troue,[1,2] Jonas Kiemle,[1,2] Hendrik Lambers,[4] Torsten Stiehm,[4] Takashi Taniguchi,[5] Kenji Watanabe,[6] Ursula Wurstbauer,[4] Andreas Knorr,[3,†] and Alexander W. Holleitner[1,2,‡]

[1] *Walter Schottky Institute and Physics Department, Technical University of Munich, Am Coulombwall 4a, 85748 Garching, Germany*
[2] *Munich Center for Quantum Science and Technology (MCQST), Schellingstr. 4, 80799 Munich, Germany*
[3] *Institut für Theoretische Physik, Nichtlineare Optik und Quantenelektronik, Technische Universität Berlin, Hardenbergstr. 36, EW 7-1, 10623 Berlin, Germany*
[4] *Institute of Physics, Münster University, Wilhelm-Klemm-Str. 10, 48149 Münster, Germany*
[5] *International Center for Materials Nanoarchitectonics, National Institute for Materials Science, Tsukuba 305-0044, Japan*
[6] *Research Center for Functional Materials, National Institute for Materials Science, Tsukuba 305-0044, Japan*

(Dated: November 29, 2024)

## I. EXPERIMENTAL DETAILS

Our heterostructures are stacked with the PDMS method on $SiO_2$/Si substrates and encapsulated with hBN. We show photoluminescence data from three different samples 1, 2 and 3 [Fig. 1(b) and Fig. S1]. All samples feature an H-type heterostructure close to 60° twist. The widths of the lowest interlayer exciton emission peak are $\gamma_1 = 3.8\,\text{meV}$, $\gamma_2 = 3.3\,\text{meV}$ and $\gamma_3 = 7.5\,\text{meV}$. All power series show the lack of an energetic blueshift, suggesting negligible interparticle interactions within the investigated range of laser power. We note that the dilute limit mentioned in the main manuscript refers to this regime of negligible interactions between interlayer excitons.

For the time-resolved photoluminescence spectra as in Fig. 4(d) of the main manuscript, we utilize a pulsed laser and a gated CCD. The detection CCD features a gate time of 2 ns. The excitation laser has a repetition rate between 150 and 201.9 kHz, which generates a time delay $\geq 4.95\,\mu\text{s}$ between pulses that far exceeds the interlayer exciton lifetime. The laser ($E_{\text{laser}} = 1.94\,\text{meV}$) has a pulse duration of 90 ps (FWHM).

* Electronic address: marten.richter@tu-berlin.de
† Electronic address: andreas.knorr@tu-berlin.de
‡ Electronic address: holleitner@wsi.tum.de

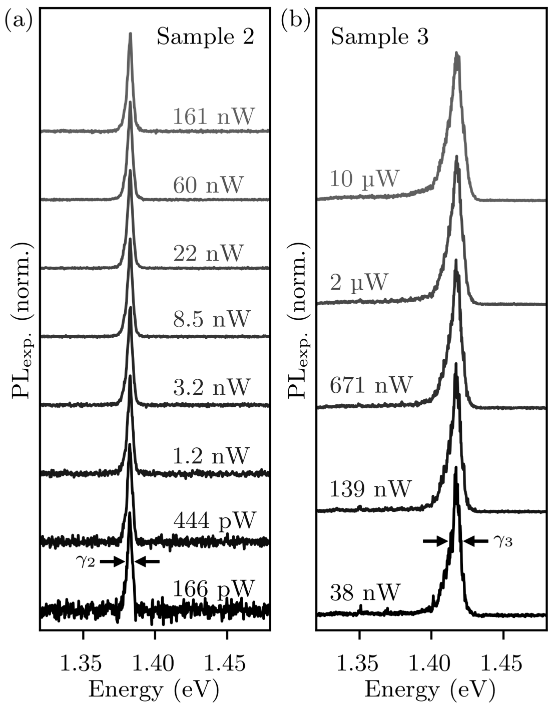


FIG. S1. Power series of experimental photoluminescence spectra on sample 2 (a) and 3 (b) at $T_{bath}^{exp} = 1.65\,K$. $\gamma_2 = 3.3\,meV$ and $\gamma_3 = 7.5\,meV$.

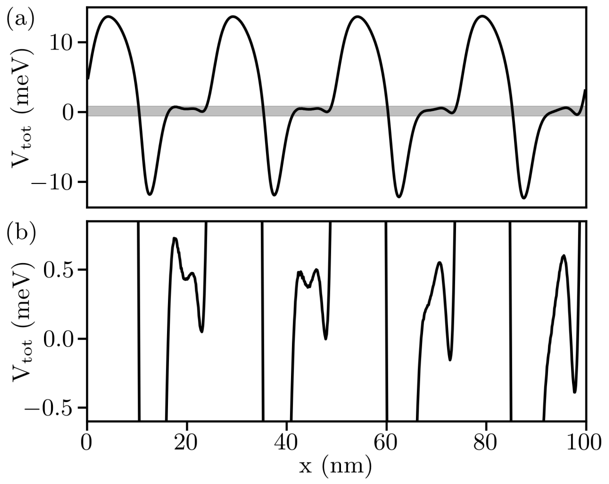


FIG. S2. (a) Cut through the potential landscape as in Fig. 2(a). (b) Enlarged presentation of the range highlighted by the grey shade in (a).

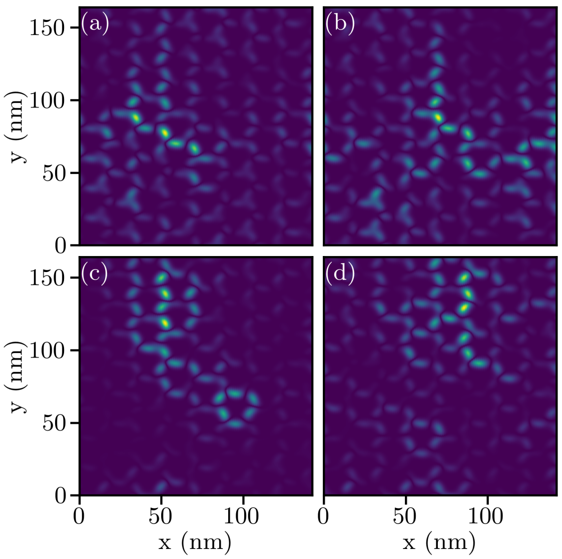


FIG. S3. Quantum wire-like states at a relative twist angle of 0.9°. Shown is $|\Psi|$ for the IX COM state with number (a) 133, (b) 135, (c) 139, and (d) 156 of 2500 calculated states.

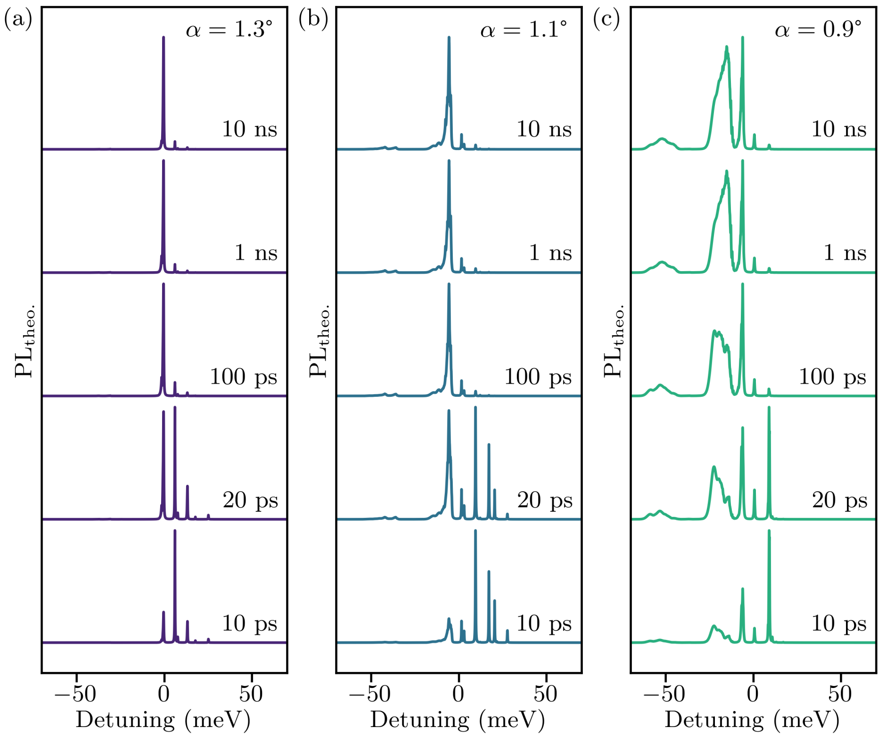


FIG. S4. Calculated photoluminescence spectra for a bilayer with a relative twist angle of 1.3° (a), 1.1° (b) and 0.9° (c) at time delays ranging from 10 ps to 10 ns with respect to the excitation pulse. The temperature is $T_{bath}^{theo} = 100\,mK$.

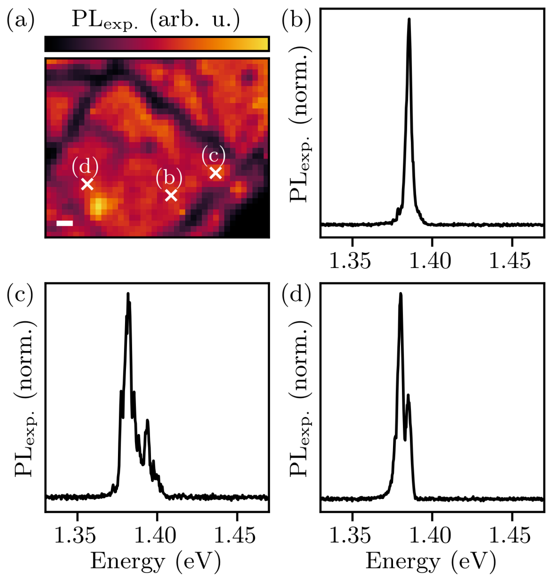


FIG. S5. (a) Experimental photoluminescence map on sample 2. The intensity is integrated in the energetic range of 1.36 and 1.4 eV. The scalebar marks 1 µm. (b-d) Normalized photoluminescence spectra at the positions indicated in (a).
